# Supplementary material for: Tuning contact line dynamics and deposition patterns in volatile liquid mixtures
Source: arXiv:1905.11211 ancillary file (2020-01-17)
Supplement: Supplementary file 1 [file supplemental.pdf]

# Tuning contact line dynamics and deposition patterns in volatile liquid mixtures – Supplemental Information

Asher P. Mouat, Clay E. Wood, Justin E. Pye, and Justin C. Burton
*Department of Physics, Emory University, Atlanta, Georgia 30322, USA*

### Supplementary Videos

**Video S1**: Partial view of an isopropanol drop spreading on a silicon wafer with ethylene glycol at $\phi = 0.001$. The playback speed is 3× real-time, and the video dimensions are 4.3 mm × 4.3 mm.

**Video S2**: Partial view of an isopropanol drop spreading on a silicon wafer with ethylene glycol at $\phi = 0.01$. The playback speed is 3× real-time, and the video dimensions are 5.5 mm × 5.5 mm.

**Video S3**: Partial view of an isopropanol drop spreading on a silicon wafer with ethylene glycol at $\phi = 0.1$. The playback speed is 3× real-time, and the video dimensions are 5.6 mm × 5.6 mm.

**Video S4**: Partial view of an isopropanol drop spreading on a silicon wafer with dodecane at $\phi = 0.1$. The playback speed is 3× real-time, and the video dimensions are 3.5 mm × 3.5 mm.

**Video S5**: Partial view of an isopropanol drop spreading on a silicon wafer with water at $\phi = 0.3$. The wafer was treated with oxygen plasma for 1 minute. The playback speed is 3× real-time, and the video dimensions are 4.7 mm × 4.7 mm.

### Thermal effects

The relevant dimensionless groups that characterize the evaporation and resulting flow in sessile drops are well-described in Ref. [1]. For the liquids used in our experiments spreading on oxidized silicon, thermal gradients and their associated effects (Marangoni, buoyancy, etc.) are small compared to solutal concentration gradients and their associated Marangoni forces. To confirm this, it is first important to realize that the silicon acts as a thermal short in the radial direction. The ratio of the thermal conductivity of the liquid ($k_{\rm l} \approx 0.14$ W/m.K, isopropanol [2]), to the thermal conductivity of the substrate ($k_{\rm s} \approx 150$ W/m.K, silicon [2]), is $k_{\rm l}/k_{\rm s} \sim 10^{-3}$. This is true for all liquids used in our experiments, and has implications for the direction of potential thermal Marangoni forces since the liquid near the contact line will be the warmest part of the drop and have the lowest surface tension [3, 4]. In this case, we expect that thermal Marangoni forces would act as a restoring force to inhibit the extension of fingers and the corresponding thin film.

Nevertheless, we can estimate the size of these effects by considering their relevant timescales. Our typical experiments last for $t_{\rm d} \approx 30$ s, when all of the solvent has evaporated away. The thermal diffusivity of the liquid and solid are $\kappa_{\rm l} = k_{\rm l}/\rho_{\rm l} c_{\rm l} \approx 6.6 \times 10^{-8}$ m$^2$/s and $\kappa_{\rm s} = k_{\rm s}/\rho_{\rm s} c_{\rm s} \approx 8.0 \times 10^{-5}$ m$^2$/s, where $\rho$ is the density and $c$ is the specific heat. In the radial direction, the drop spreads to a maximum radius of $R_{\rm max} \approx 5$ mm. Thus the time scale for thermal equilibriation in the silicon is $t_{\rm s} \approx R_{\rm max}^2/\kappa_{\rm s} = 0.3$ s. Inside the drop, heat also diffuses in the vertical direction. Assuming a maximum drop thickness at the initiation of spreading of $h_0 \approx 100$ $\mu$m, the time scale for thermal equilibriation in the liquid is $t_{\rm l} \approx h_0^2/\kappa_{\rm l} = 0.15$ s. Both of these timescales are much smaller than $t_{\rm d} \approx 30$ s. The drop will be in thermal equilibrium if the evaporation is rate-limited by the diffusion of solvent vapor above the drop. An upper bound for the diffusivity of vapor is $\kappa_{\rm v} \approx 10^{-5}$ m$^2$/s. The mass flux is occurring over a length scale $R_{\rm max}$. Thus the timescale for vapor diffusion is $t_{\rm v} \approx R_{\rm max}^2/\kappa_{\rm v} = 2.5$ s, which is 10 times slower than vertical thermal diffusion in the liquid.

Moreover, we can directly compare the effects of thermal surface tension and density gradients to solutal ones using the Marangoni number (Ma) and buoyancy number (Bu). The Marangoni number is the ratio of flow velocity induced by Marangoni stress to the mass-loss velocity [1]:

$$\mathrm{Ma} = -\frac{d\gamma^{\rm lv}}{dT}\frac{\Delta T t_{\rm d} h_0}{\eta_{\rm l} R_{\rm max}^2}, \tag{1}$$

where $d\gamma^{\rm lv}/dT$ is the slope of the liquid-vapor surface tension variation with temperature, $\Delta T$ is the maximum temperature gradient in the radial direction, and $\eta_{\rm l}$ is the dynamic liquid viscosity. A reasonable estimate for $\Delta T$ can be found by the maximum change in temperature of the silicon after the solvent has fully evaporated, $\Delta T = L_{\rm l}\rho_{\rm l} V_{\rm l}/c_{\rm s}\rho_{\rm s} V_{\rm s}$, where $L_{\rm l}$ is the latent heat of the liquid, and $V_{\rm l}$ ($V_{\rm s}$) is the volume of the liquid (solid). Using values for the isopropanol and the silicon wafer (thickness $h_{\rm s} = 500$ $\mu$m) immediately below the drop: $L_{\rm l} = 6.7\times 10^5$ J/kg, $\rho_{\rm l} = 790$ kg/m$^3$, $V_{\rm l} = 1$ $\mu$l, $c_{\rm s} = 2680$ J/kg.K, $\rho_{\rm s} = 2320$ kg/m$^3$, and $V_{\rm s} = \pi R_{\rm max}^2 h_{\rm s} = 3.9 \times 10^{-8}$ m$^3$, we estimate that $\Delta T \approx 2$ K.

The Marangoni number can now be computed using $d\gamma^{\rm lv}/dT = -1.3 \times 10^{-4}$ N/m.K and $\eta_{\rm l} = 2.1$ mPa.s for isopropanol [2], and $h_0 = $ 10-100 $\mu$m in the experiments.

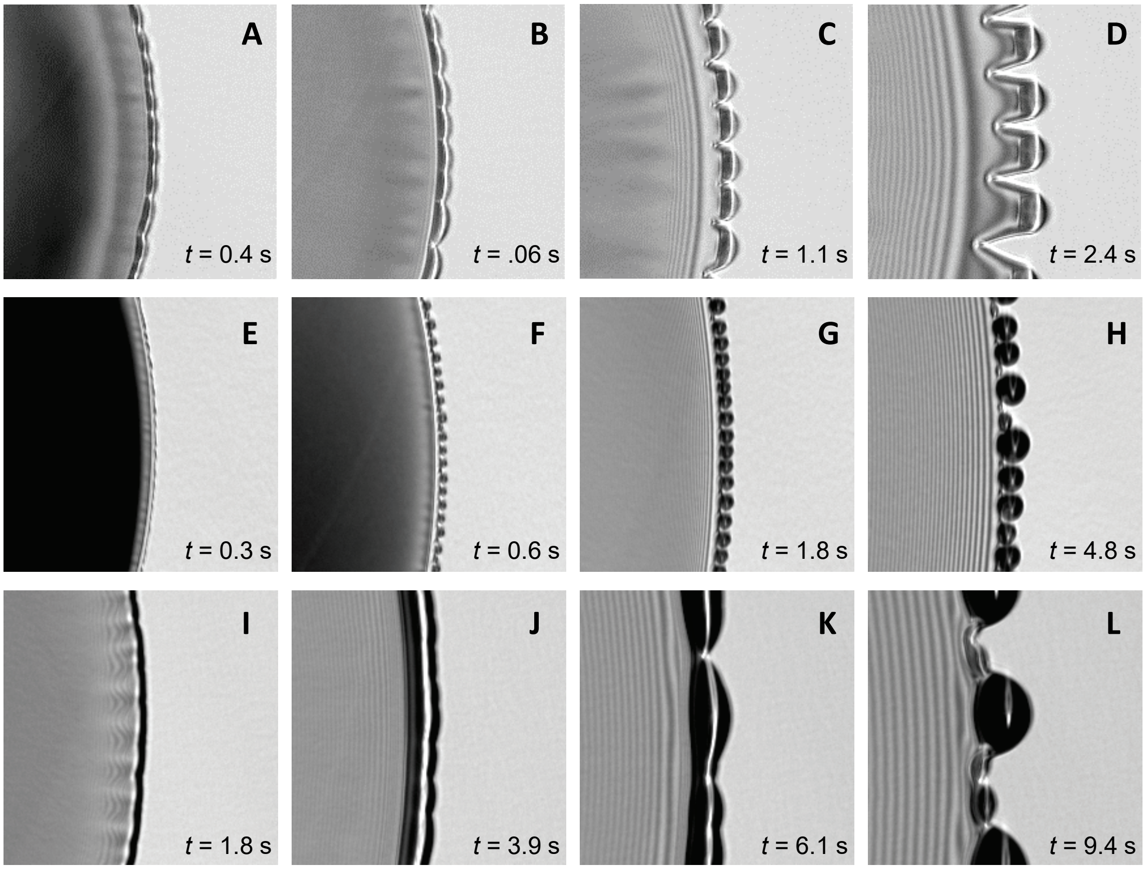


FIG. S1. Time series of the contact line region for an isopropanol drop with ethylene glycol at $\phi = 0.1$ (**A-D**), dodecane at $\phi = 0.1$ (**E-F**), and glycerol at $\phi = 0.1$ (**I-L**), spreading on a silicon surface. The size of all images is 1 mm × 1 mm. The solute rim that develops at early times breaks up into droplets.

The result is that Ma = 1-10. This is more than 2 orders of magnitude smaller than in situations where thermal Marangoni forces are important [1]. Additionally, this is an upper bound that assumes diffusion is the only thermal transport mechanism. In fact, advection of the fluid during spreading in our experiments is more rapid than diffusion, and helps to reduce temperature gradients. We can also estimate the effects of thermally-induced convection through the buoyancy number:

$$\mathrm{Bu} = \frac{g\beta\Delta T h_0^2 t_\mathrm{d} \rho_\mathrm{l}}{\eta_\mathrm{l} R_\mathrm{max}}, \tag{2}$$

where $g$ is the acceleration due to gravity and $\beta$ is the volumetric thermal expansion coefficient. Using $\beta = 1.1\times10^{-3}\ \mathrm{K}^{-1}$ for isopropanol and the parameters above, we estimate that $0.005 < \mathrm{Bu} < 0.5$, which is again more than 2 orders of magnitude smaller than typical experiments where convection is important.

Finally, we can directly compare the role of thermal and solutal effects in our experiments by taking the ratio of driving forces. The largest surface tension difference due to thermal gradients is estimated as $-\Delta T \times d\gamma^\mathrm{lv}/dT \approx 0.25$ mN/m. The maximum solutal surface tension difference with isopropanol is $\sim$ 2-50 mN/m, a range bounded by dodecane and water. For buoyancy effects, the normalized density difference between warm and cold regions of the isopropanol is $\beta\Delta T \approx 2.2\times10^{-3}$, and the smallest solutal density difference is between isopropanol (790 kg/m$^3$) and dodecane (750 kg/m$^3$): (790-750)/790 = $5.0\times10^{-2}$. In both cases, solutal driving forces are more than an order of magnitude stronger than thermal driving forces.

### Rim formation and breakup

The rapid spreading and evaporation near the contact line leads to a build-up of solute in this region. Since the partially-wetting solute doesn't evaporate appreciably on the timescale of the experiment, a thick, toroidal rim of solute will form at the contact line, and be pushed outward radially with the spreading solvent. This rim is subject to the Rayleigh-Plateau instability, and will eventually develop thickness variations as it begins to break up into droplets [5]. Further evolution of the droplets will depend on the threshold specified in Eq. 1 of the

main text. If Marangoni forces are above the threshold to initiate fingers, then the thick regions, where the solute concentration and surface tension is highest, will extend faster than the main drop.

Figure S1 shows the evolution of the rim for an isopropanol drop with ethylene glycol at $\phi = 0.1$. The fastest-growing wavelength for the Rayleigh-Plateau instability in an inviscid fluid is $\Lambda_c \approx 4.01a$ [5], where $a$ is the characteristic thickness of the rim. For a viscous fluid, the longest wavelengths are the most unstable. The Ohnesorge number, which measures the ratio of viscous to inertial and surface tension forces, is defined as:

$$\mathrm{Oh} = \frac{\mu}{\sqrt{\gamma \rho a}}. \tag{3}$$

For Oh $\ll 1$, the rim should behave as an inviscid fluid. At 22°C, the viscosity of ethylene glycol at 22°C is 16.0 mPa.s, and its density is 1100 kg/m$^3$. From Fig. S1B, we estimate that $a \approx 50$ $\mu$m. Thus, for ethylene glycol, Oh $\sim 0.3$. We would then expect that the characteristic wavelength for the undulations seen in Fig. S1A-B during the early stages of the instability should be of order $4a$, which seems to be in good agreement. These undulations eventually pull away from the main drop and form well-defined fingers, as shown in Fig. S1C-D. However, the length $L$ and wavelength $\Lambda$ continue to grow since they are continually fed with liquid from the spreading drop.

For dodecane, fingers do not form because Marangoni forces are not strong enough (Eq. 1, main text). In this case, the Rayleigh-Plateau instability produces well-defined pearls instead of fingers. At 22°C, the viscosity of dodecane is 1.36 mPa.s, and its density is 750 kg/m$^3$. Due to dodecane's low viscosity, the Rayleigh-Plateau instability evolves faster, and the droplets are produced at early times (Fig. S1E-F). If we use $a \approx 10$ $\mu$m, then we estimate Oh $\sim 0.1$ for dodecane. The spacing and diameter of the drops seen in Fig. S1F agree reasonably well with the inviscid theory. The well-defined drops continue to grow and the pattern coarsens due to the coalescence of neighboring drops, as shown in Fig. S1G-H.

Glycerol has a much higher viscosity than the other fluids in our experiments (1180 mPa.s), thus the evolution of the instability is much slower, and takes place when the rim is thicker at later times. As shown in Fig. S1I-J, a thick rim ($a \approx 150$ $\mu$m) still exists 3.9 s after deposition. The density of glycerol is 1260 kg/m$^3$, so Oh $\sim 10$. Nevertheless, the inviscid theory still seems to hold reasonably well, and $\Lambda_c \approx 600$ $\mu$m. In this case, glycerol's larger contact angle inhibits surface wetting, despite the strong solutal Marangoni forces, so pearls are formed instead of fingers (Fig. S1K-L).

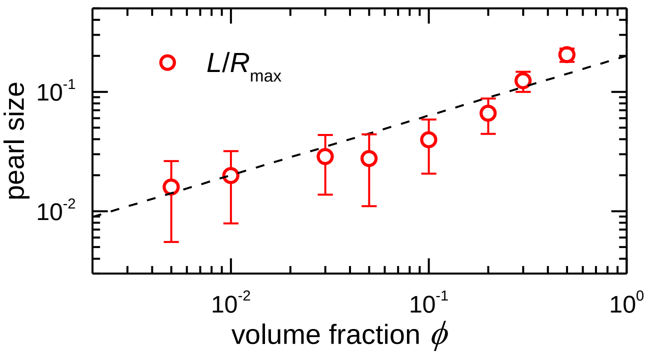


FIG. S2. Normalized pearl length vs. solute volume fraction for isopropanol drops spreading with dodecane at different concentrations. The dashed line represents $\phi^{1/2}$.

### Drop deposition from pearl-forming mixtures

For solutes that formed pearls while spreading, isolated drops were deposited on the surface as the contact line receded. The patterns formed by the drops depended strongly on the solute properties, concentration, and the evaporative conditions (i.e. local isopropanol vapor concentration). The size of the pearls, characterized by their normalized length, $L/R_{\mathrm{max}}$, decreased with concentration in a similar fashion as ethylene glycol (Fig. 1C-F). This is shown in Fig. S2. The scaling generally consistent with $L/R_{\mathrm{max}} \propto \phi^{1/2}$, although there is much more variation in the data since pearls can coalesce as they spread outward. Figure S3 shows a few examples of the different patterns observed. Many of these patterns have been discussed previously for the evaporative deposition of colloids or polymer films [1, 6–10].

For drops with low concentrations and low-viscosity solutes, small drops were deposited in multiple stages. Figure S3A-C shows a drop with dodecane at $\phi = 0.005$. There are two concentric rings of drops resulting from a two-stage receding mechanism. In S3B, drops are emitted directly from the contact line, whereas in S3C, drops are emitted prior to the edge of the isopropanol film and "glide" towards the edge. This deposition pattern (ring-like structures near the edge and a solid circle near the center), is discussed in detail in Wu et al. [8] for colloidal particles.

For higher concentrations of dodecane, as shown in Fig. S3D-F, large drops are deposited on the surface and remain quite spherical until the isopropanol vapor has had time to diffuse. As mentioned previously, this will occur over $t_{\mathrm{v}} \approx R_{\mathrm{max}}^2/\kappa_{\mathrm{v}} = 2.5$ s, at the very least. Similar patterns are formed for higher-viscosity solutes. Figure S3G-I shows an isopropanol drop with glycerol at $\phi = 0.05$. The deposition pattern is similar to dodecane, but in general, for a given fixed concentration, larger viscosity produces larger drops. This may be expected since

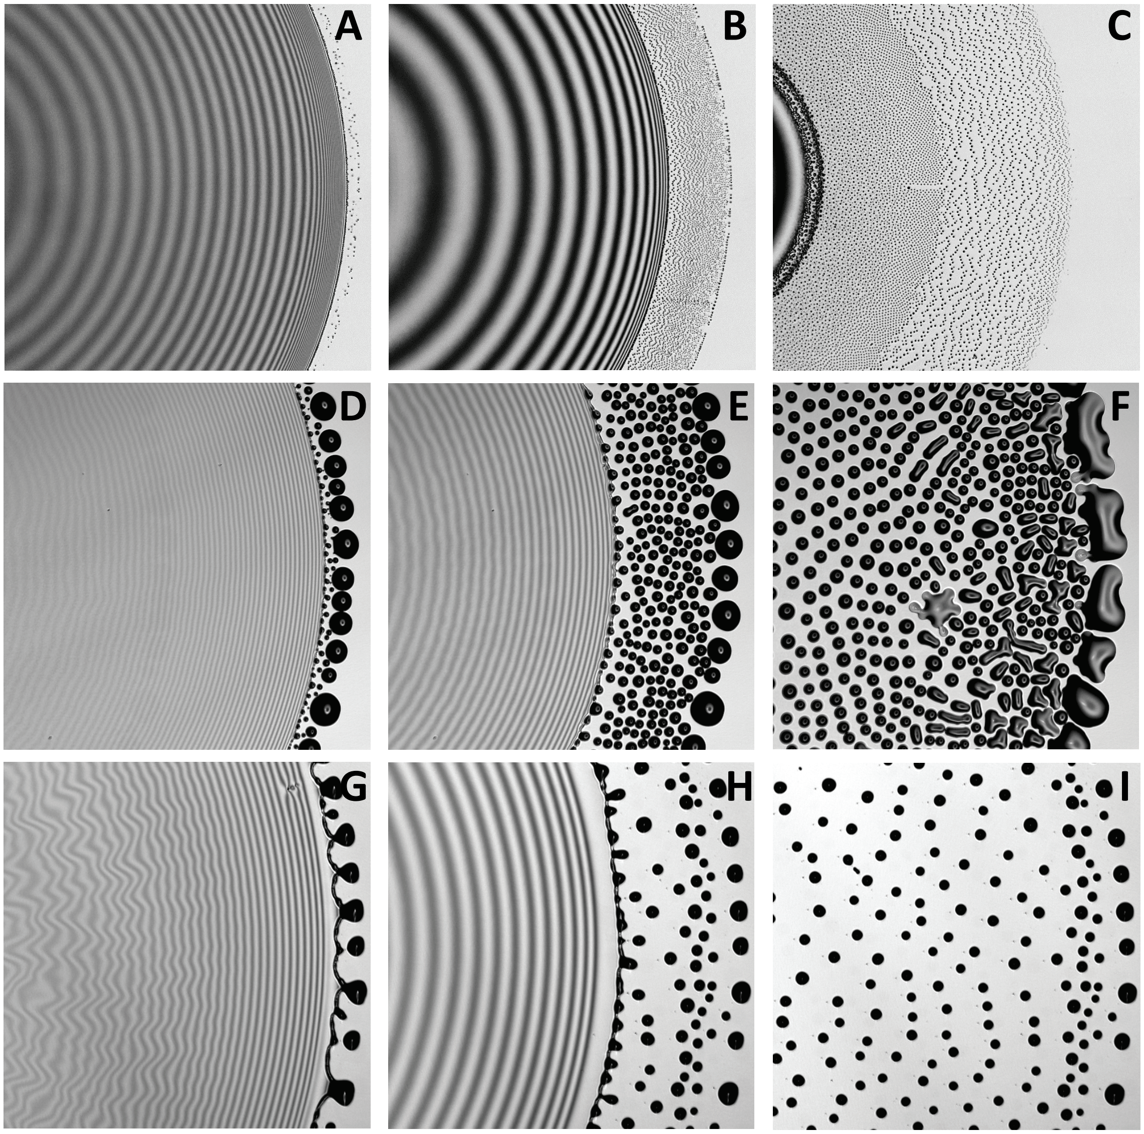


FIG. S3. (**A-C**) Time series of an isopropanol drop with dodecane at $\phi = 0.005$ spreading on a silicon surface. The small drops are deposited from the receding contact line. The time from deposition for each frame is 10.2 s, 17.5 s, and 23.2 s. The drops at the maximum radius have started to evaporate in **C**. (**D-F**) Time series of an isopropanol drop with dodecane at $\phi = 0.2$ spreading on a silicon surface. Large drops begin to wet the surface as the isopropanol diffuses away. The time from deposition for each frame is 11.4 s, 22.6 s, and 40.0 s. (**G-I**) Time series of an isopropanol drop with glycerol at $\phi = 0.05$ spreading on a silicon surface. The time from deposition for each frame is 11.9 s, 19.6 s, and 24.8 s. The size of all images is 3 mm $\times$ 3 mm.

the time for a single drop to form and pinch-off from the receding film will increase with viscosity.


[1] R. G. Larson, Transport and deposition patterns in drying sessile droplets, AIChE Journal **60**, 1538 (2014).

[2] *CRC Handbook of Chemistry and Physics, 99th Edition*, 99th ed. (CRC Press, 2018).

[3] W. D. Ristenpart, P. G. Kim, C. Domingues, J. Wan, and H. A. Stone, Influence of substrate conductivity on circulation reversal in evaporating drops, Phys. Rev. Lett. **99**, 234502 (2007).

[4] S. Karpitschka, F. Liebig, and H. Riegler, Marangoni contraction of evaporating sessile droplets of binary mixtures, Langmuir **33**, 4682 (2017).

[5] J. Eggers, Nonlinear dynamics and breakup of free-surface flows, Rev. Mod. Phys. **69**, 865 (1997).

[6] C. N. Kaplan, N. Wu, S. Mandre, J. Aizenberg, and L. Mahadevan, Dynamics of evaporative colloidal patterning, Phys. Fluids **27**, 092105 (2015).

[7] M. Gonuguntla and A. Sharma, Polymer patterns in evaporating droplets on dissolving substrates, Langmuir **20**, 3456 (2004).

[8] M. Wu, X. Man, and M. Doi, Multi-ring deposition pattern of drying droplets, Langmuir **34**, 9572 (2018).

[9] Z. Lin and S. Granick, Patterns formed by droplet evaporation from a restricted geometry, J. Am. Chem. Soc. **127**, 2816 (2005).
[10] R. D. Deegan, O. Bakajin, T. F. Dupont, G. Huber, S. R. Nagel, and T. A. Witten, Contact line deposits in an evaporating drop, Phys. Rev. E **62**, 756 (2000).
